# Supplementary material for: Policy Gradient for Continuing Tasks in Non-stationary Markov Decision Processes
Source: arXiv:2010.08443 source file (2020-10-16)
Supplement: Supplementary file 1 [file appendix_komp.tex]

\subsection{Kernel Orthogonal Matching Pursuit}\label{sec_komp}
In this section we present the details of Kernel Orthogonal Matching Pursuit. Starting with the policy $h_0 \equiv 0$, each stochastic gradient ascent iteration  defines a new policy
\begin{equation}\label{eqn_partial_grad_ascent}
\tilde{h}_{k+1} = h_k +\eta\hat{\nabla}_h U_{s_k}(h_k,\cdot),
  \end{equation}
where $\hat{\nabla}_h U_{s_k}(h_k,\cdot)$ is that in \eqref{eqn_stochastic_gradient}. 
The difference between the updates \eqref{eqn_partial_grad_ascent} and  \eqref{eqn_stochastic_update}   is that in \eqref{eqn_partial_grad_ascent} $h_k=\sum_{j=1}^{M_k} \kappa(s_{T^j}^{(k)},\cdot)w_j^{(k)}$ is represented by a reduced $M_k\leq k$ number of states $s_{T^j}^{(k)}$ and weights $w_j^{(k)}\in\mathbb{R}^p$, as it results from the pruning procedure below, (cf., $M_k=k$ for $h_{k+1}$ in \eqref{eqn_stochastic_update}).
Let $(s_{T^k},a_{T^k})$ be the state-action pair $(s_T, a_T) $ in step 7 Algorithm \ref{alg_stochastic_grad} at its $k$--th call by Algorithm \ref{alg_online_policy_gradient}. Then define
\begin{equation}\label{eqn_weights}
  \tilde{w}_k :=\eta \frac{\hat{Q}(s_{T^k},a_{T^k};h_k)}{1-\gamma}\Sigma^{-1}(a_{T^k}-h_k(s_{T^k})),
\end{equation}
and rewrite $\eta\hat{\nabla}_h U_{s_k}(h_k,\cdot)$ using the expression  \eqref{eqn_stochastic_gradient} and \eqref{eqn_weights} as $\eta\hat{\nabla}_h U_{s_k}(h_k,\cdot) = \kappa(s_{T_k},\cdot)\tilde{w}_k$. Thus, we can write $\tilde{h}_{k+1}$
\begin{equation}
\tilde{h}_{k+1} = \sum_{j=1}^{M_{k}}  \kappa(s_{T^j}^{(k)},\cdot)w_j^{(k)}+\kappa(S_{T^k},\cdot)\tilde{w}_k.
\end{equation}
Hence, $h_k$ is represented by dictionary $D_k=[s_{T^k}^{(k)},\ldots, s_{T^{M_k}}^{(k)}]$ and associated weights $\bbw_k=\left[\left(w_1^{(k)}\right)^\top,\ldots,\left(w_{M_k}^{(k)}\right)^\top\right]^\top,$ and 
%
%where $M_{k}\leq k$ is the number of elements in the kernel dictionary needed to represent the function ${h}_{k}$. 
%
 $\tilde{h}_{k+1}$ is represented by the  updated  $\tilde{D}_{k+1} = [D_k, s_{T_k}]$ and $\tilde{\bbw}_{k+1} = [\bbw_k^\top, \tilde{w}_{k}^\top]^\top$, which has model order $\tilde{M}_{k+1} = M_k+1$. Then, to avoid memory explosion, we prune the dictionary as long as the induced error stays below a prescribed bound $\epsilon>0$. 
We start by storing copies of the previous dictionary, i.e., define ${D}_{k+1} = \tilde{D}_{k+1}$ and ${\bbw}_{k+1} = \tilde{\bbw}_{k+1}$. Let $\ccalH_{{D}^j_{k+1}}$ be the space spanned by all the elements of ${D}_{k+1}$ except for the $j$-th one. For each $j=1 \ldots {M}_{k+1}$ we identify the less informative dictionary element by solving
%
%\begin{equation}\label{eqn_pruning_optimization}
%  \begin{split}
%    e_j &= \min_{{h}\in\ccalH_{\tilde{D}^j_{k+1}}}\left\| {h}-\tilde{h}_{k+1}\right\|_\ccalH^2\\
%   & = \min_{\bbw \in \mathbb{R}^{p M_k}}
%    \bbw^\top \bbK_{\tilde{D}^j_{k+1},\tilde{D}^j_{k+1}} \bbw -2 \bbw^\top \bbK_{\tilde{D}^j_{k+1},{D}_{k+1}}\tilde{\bbw}_{k+1} \\
%    &\phantom{\argmin_{\bbw \in \mathbb{R}^{p M_k}}}+ \tilde{\bbw}_{k+1}^\top \bbK_{{D}_{k+1},{D}_{k+1}}\tilde{\bbw}_{k+1},
%\end{split}
%\end{equation}
\begin{align}\label{eqn_pruning_optimization}
    e_j &= \min_{{h}\in\ccalH_{{D}^j_{k+1}}}\left\| {h}-\tilde{h}_{k+1}\right\|_\ccalH^2  =\tilde{\bbw}_{k+1}^\top \bbK_{\tilde{D}_{k+1},\tilde{D}_{k+1}}\tilde{\bbw}_{k+1}\\
   & +\hspace{-0.1cm} \min_{\bbw \in \mathbb{R}^{p M_{k+1}-1}}\hspace{-0.1cm}
    \bbw^\top \bbK_{{D}^j_{k+1},{D}^j_{k+1}} \bbw -2 \bbw^\top \bbK_{{D}^j_{k+1},\tilde{D}_{k+1}}\tilde{\bbw}_{k+1}, \nonumber 
\end{align}
%
%which results from expanding the square after substituting $h$ and $\tilde{h}_{k+1}$ by its representation as weighted sums of kernel elements and upon defining the block matrices $\bbK_{\tilde{D}^j_{k+1},\tilde{D}^j_{k+1}}$ whose $(i,l)$ block of size $p\times n$ is $\kappa((\tilde{D}^j_{k+1})_i,(\tilde{D}^j_{k+1})_l)$, \red{respectively for $\bbK_{\tilde{D}^j_{k+1},{D}_{k+1}}$ and $\bbK_{{D}_{k+1},{D}_{k+1}}$} \blue{not happy with this. Juan?} The previous problem is a least-squares problem and it has the following closed form solution 
%
%
  which results from expanding the square after substituting $h$ and $\tilde{h}_{k+1}$ by their representations as weighted sums of kernel elements, and upon defining the block matrices $\bbK_{\tilde{D}_{k+1},\tilde{D}_{k+1}}$, $\bbK_{{D}^j_{k+1},{D}^j_{k+1}}$ and $\bbK_{{D}^j_{k+1},\tilde{D}_{k+1}}$ as block matrices whose $(l,m)$-th blocks of size $p\times p$ are $\kappa\left(\tilde{s}_{T^l}^{(k)},\tilde{s}_{T^m}^{(k)}\right)$, $\kappa\left(s_{T^l}^{(k)},s_{T^m}^{(k)}\right)$ and $\kappa\left(s_{T^l}^{(k)},\tilde{s}_{T^m}^{(k)}\right)$, where $s_{T^i}^{(k)}$ and $\tilde{s}_{T^i}^{(k)}$ correspond to the $i$-th element of $D_{k+1}^j$ and of $\tilde{D}_{k+1}$ respectively.
%
%%%%%%%%%%%%%%%%%%%%%%%%%%%%%%%%%%%%%%%%%%%%%%%%%%%%%%%%%%%%%%%%%%%%%%%%%%%%%%%%%%%%%%%%%%%%%%%%%%%%%%%%%%%%%%%%%%%%%%%%%%% A L G O R I T H M %%%%%%%%%%%%%%%%%%%%%%%%%%%%%%%%%%%%%%%%%%%%%%%%%%%%%%%%%%%%%%%%%%%%%%%%%%%%%%%%%%%%%%%%%%%%%%%%%%%%%%%%%%%%%%%%%%%%%%%%%%%%%%%%%%%%%%%%%%%%%%%%%%%%%%%%%%%%%%%
\begin{algorithm}
 \caption{Kernel Orthogonal Matching Pursuit (KOMP)}
\begin{algorithmic}[1]

 \Require function ${\tilde{h}_k}$ defined by Dictionary $\tilde{D}_k\in\mathbb{R}^{n\times \tilde{M}_k}$ weights $\tilde{\bbw}_k\in\mathbb{R}^{p \times \tilde{M}_k}$ and compression budget $\epsilon>0$
 \State \textit{Initialize}: ${D}_k = \tilde{D}_k$, $\bbw_k=\tilde{\bbw}_k$, $M_k=\tilde{M}_k$, $e^\star=0$
 \While{$e^\star<\epsilon$ and $M_k>0$}
 \For{$j=1\ldots {M}_k$}
 \State Find minimal error $e_j$ by solving \eqref{eqn_pruning_optimization}
 \EndFor
  \State Less informative element $j^\star = \argmin_{j} e_j$ 
  %  \State Find less informative dictionary element $j^\star = \argmin_{j=1\ldots M_k} e_j$
  \State Save error $e^\star = e_{j^\star}$
  \If{Error smaller than compression budget $e^\star <\epsilon$}
  \State Prune Dict., ${D}_{k} \leftarrow {D}_{k}^{j^\star} $, ${M}_k \leftarrow {M}_k-1$
  \State Update Weights as in \eqref{eqn_least_square_solution}
  $$
{\bbw}_k =  \bbK_{{D}_{k},{D}_{k}}^\dagger \bbK_{{D}_{k},\tilde{D}_{k}}\tilde{\bbw}_{k}
 $$
  \EndIf
  \EndWhile\\
 \Return ${D}_k,{\bbw}_k$ 
 \end{algorithmic}\label{algorithm_komp}
 \end{algorithm}
%
%%%%%%%%%%%%%%%%%%%%%%%%%%%%%%%%%%%%%%%%%%%%%%%%%%%%%%%%%%%%%%%%%%%%%%%%%%%%%%%%%%%%%%%%%%%%%%%%%%%%%%%%%%%%%%%%%%%%%%%%%%%%%%%%%%%%%%%%%%%%%%%%%%%%%%%%%%%%%%%%%%%%%%%%%%%%%%%%%%%%%%%%%%%%%%%%%%%%%%%%%%%%%
%
Problem \eqref{eqn_pruning_optimization} is a least-squares problem with the following closed-form solution 
\begin{equation}\label{eqn_least_square_solution}
\bbw^\star_j = \bbK_{{D}^j_{k+1},{D}^j_{k+1}}^\dagger \bbK_{{D}^j_{k+1},\tilde{D}_{k+1}}\tilde{\bbw}_{k+1},
  \end{equation}
where, $\left(\cdot\right)^\dagger$ denotes the Moore-Penrose pseudo-inverse. After computing all compression errors $e_j$ we chose the dictionary element that yields the smallest error $j^\star = \argmin_{j=1 \ldots M_{k+1}} e_j$, we remove the $j^\star$-th column from the dictionary ${D}_{k+1}$, i.e., we redefine ${D}_{k+1} = {D}_{k+1}^{j^\star}$ and the model order $M_{k+1} =M_{k+1}-1$ and update the corresponding weights as ${\bbw}_{k+1} = \bbw^\star_{j^\star}$. We repeat the process as long as the minimum compression error remains below the compression budget, i.e.,  $\min_{j=1 \ldots M_{k+1}} e_j<\epsilon$. The output of the pruning process is a function $h_{k+1}$ that is represent by at most the same number of elements than $\tilde{h}_{k+1}$ and such that the error introduced in this approximation is, by construction, smaller than the compression budget $\epsilon$. This output can be interpreted as a projection over a RKHS of smaller dimension. Let $D_{k+1}$ be the dictionary that Algorithm \ref{algorithm_komp} outputs. Then, the resulting policy can be expressed as 
\begin{equation}\label{eqn_proj_stochastic_ascent}
\hspace{-.1cm}h_{k+1}\hspace{-.1cm} =\hspace{-.1cm} \ccalP_{\ccalH_{D_{k+1}}}\hspace{-.1cm}\left[ \tilde{h}_{k+1}\right]\hspace{-.1cm} =\hspace{-.1cm} \ccalP_{\ccalH_{D_{k+1}}}\hspace{-.1cm}\left[h_{k}+\eta \hat{\nabla}_h U_{s_k}(h_k,\cdot)\right],
\end{equation}
where the operation $\ccalP_{\ccalH_{D_{k+1}}}\left[ \cdot \right]$ refers to the projection onto the RKHS spanned by the dictionary $D_{k+1}$.
